# Supplementary material for: Cross Device Federated Intrusion Detector for Early Stage Botnet Propagation in IoT
Source: arXiv:2311.08621 source file (2023-11-15)
Supplement: Supplementary file 1 [file A1.tex]

% \chapter{Sample Appendix}

% Include data here and other details that fit appropriately in an Appendix.

% You may have as many appendices as necessary, simply follow this one as a template for including more.
